# Supplementary material for: Enhanced spin-orbit coupling and orbital moment in ferromagnets by electron correlations
Source: arXiv:2106.01046 source file (2021-06-02)
Supplement: Supplementary file 1 [file supplementary_information.pdf]

# Supplementary information for "Enhanced spin-orbit coupling and orbital moment in ferromagnets by electron correlations"

Ze Liu,[1] Jing-Yang You,[2] Bo Gu,[1,3,*] Sadamichi Maekawa,[4,1] and Gang Su[1,3,5,†]

[1]*Kavli Institute for Theoretical Sciences, and CAS Center for Excellence in Topological Quantum Computation, University of Chinese Academy of Sciences, Beijing 100190, China*

[2]*Department of Physics, National University of Singapore, 2 Science Drive 3, Singapore 117551*

[3]*Physical Science Laboratory, Huairou National Comprehensive Science Center, Beijing 101400, China*

[4]*Center for Emergent Matter Science, RIKEN, Walo 351-0198, Japan*

[5]*School of Physical Sciences, University of Chinese Academy of Sciences, Beijing 100049, China*

## I. TWO-ORBITAL HUBBARD MODEL WITH SPIN-ORBIT COUPLING

The Hamiltonian of multi-orbital Hubbard model with the spin-orbit coupling (SOC) is written as

$$H = \sum_{\mathbf{k},m,\sigma} \epsilon_{\mathbf{k}m\sigma} n_{\mathbf{k}m\sigma} + U \sum_{i,m} n_{im\uparrow} n_{im\downarrow} + \frac{U'}{2} \sum_{i,m\neq m',\sigma,\sigma'} n_{im\sigma} n_{im'\sigma'} - \frac{J_H}{2} \sum_{i,m\neq m',\sigma} n_{im\sigma} n_{im'\sigma}, \tag{1}$$

where $\epsilon_{\mathbf{k}m\sigma}$ is the energy for electron with wave vector $\mathbf{k}$, orbital $m$, and spin $\sigma$ ($\uparrow,\downarrow$), $U$ is the on-site Coulomb repulsion within the orbital $m$, $U'$ is the on-site Coulomb repulsion between different orbitals $m$ and $m'$, and $J_H$ is the Hund coupling. $n_{\mathbf{k}m\sigma}(n_{im\sigma})$ represents the particle number of electron with wave vector $\mathbf{k}$ (site index $i$), orbital $m$ and spin $\sigma$. As a simple model to describe the ferromagnetic metals with SOC, we consider the two-orbital Hubbard model, where only a pair of opposite orbitals is included (as $m = 1, -1$ or $m = 2, -2$ for transition metals). Thus, the Hamiltonian can be simplified as

$$H = \sum_{\mathbf{k},m,\sigma} \epsilon_{\mathbf{k}m\sigma} n_{\mathbf{k}m\sigma} + U \sum_{i,m} n_{im\uparrow} n_{im\downarrow} + U' \sum_{i,\sigma,\sigma'} n_{im\sigma} n_{i\bar{m}\sigma'} - J_H \sum_{i,\sigma} n_{im\sigma} n_{i\bar{m}\sigma}. \tag{2}$$

For simplicity, we consider four degenerate energy bands, which are lifted by external magnetic field $h$ and the Ising-type SOC[1]

$$\epsilon_{\mathbf{k}m\sigma} = \epsilon_{\mathbf{k}} - \sigma\mu_B h - \frac{1}{2}\sigma\lambda_{so} m, \tag{3}$$

where $\lambda_{so}$ is the SOC constant, $\epsilon_{\mathbf{k}}$ is the electron energy without the external magnetic filed and SOC. Using the Hartree-Fock approximation

$$n_{im\sigma} n_{im'\sigma'} \approx \langle n_{im\sigma} \rangle n_{im'\sigma'} + \langle n_{im'\sigma'} \rangle n_{im\sigma} - \langle n_{im\sigma} \rangle \langle n_{im'\sigma'} \rangle, \tag{4}$$

the interaction terms can be written separately as:

$$\begin{aligned}
n_{im\uparrow} n_{im\downarrow} &\approx \langle n_{im\uparrow} \rangle n_{im\downarrow} + \langle n_{im\downarrow} \rangle n_{im\uparrow} - \langle n_{im\uparrow} \rangle \langle n_{im\downarrow} \rangle, \\
n_{i\bar{m}\uparrow} n_{i\bar{m}\downarrow} &\approx \langle n_{i\bar{m}\uparrow} \rangle n_{i\bar{m}\downarrow} + \langle n_{i\bar{m}\downarrow} \rangle n_{i\bar{m}\uparrow} - \langle n_{i\bar{m}\uparrow} \rangle \langle n_{i\bar{m}\downarrow} \rangle, \\
n_{im\uparrow} n_{i\bar{m}\uparrow} &\approx \langle n_{im\uparrow} \rangle n_{i\bar{m}\uparrow} + \langle n_{i\bar{m}\uparrow} \rangle n_{im\uparrow} - \langle n_{im\uparrow} \rangle \langle n_{i\bar{m}\uparrow} \rangle, \\
n_{im\downarrow} n_{i\bar{m}\downarrow} &\approx \langle n_{im\downarrow} \rangle n_{i\bar{m}\downarrow} + \langle n_{i\bar{m}\downarrow} \rangle n_{im\downarrow} - \langle n_{im\downarrow} \rangle \langle n_{i\bar{m}\downarrow} \rangle, \\
n_{im\uparrow} n_{i\bar{m}\downarrow} &\approx \langle n_{im\uparrow} \rangle n_{i\bar{m}\downarrow} + \langle n_{i\bar{m}\uparrow} \rangle n_{im\downarrow} - \langle n_{im\uparrow} \rangle \langle n_{i\bar{m}\downarrow} \rangle, \\
n_{im\downarrow} n_{i\bar{m}\uparrow} &\approx \langle n_{im\downarrow} \rangle n_{i\bar{m}\uparrow} + \langle n_{i\bar{m}\downarrow} \rangle n_{im\uparrow} - \langle n_{im\downarrow} \rangle \langle n_{i\bar{m}\uparrow} \rangle.
\end{aligned} \tag{5}$$

Assuming the system is uniform, and the occupation number $n_{im\sigma}$ is independent of lattice site $i$,

$$\langle n_{im\sigma} \rangle \approx \langle n_{m\sigma} \rangle, \tag{6}$$

and making the Fourier transformation:

$$\sum_i n_{im\sigma} = \sum_{\mathbf{k}} n_{\mathbf{k}m\sigma}, \tag{7}$$

the Hamiltonian in Eq.(2) can be diagonalized as

$$H \approx \sum_{\mathbf{k},m,\sigma} \tilde{\epsilon}_{\mathbf{k}m\sigma} n_{\mathbf{k}m\sigma}, \tag{8}$$

with

$$\tilde{\epsilon}_{km\sigma} = \epsilon_k - \sigma\mu_B h - \frac{1}{2}\sigma\lambda_{so} m + U \langle n_{m\bar{\sigma}} \rangle + U' (\langle n_{\bar{m}\sigma} \rangle + \langle n_{\bar{m}\bar{\sigma}} \rangle) - J_H \langle n_{\bar{m}\sigma} \rangle. \tag{9}$$

The spin polarization per site is defined as

$$s_z = \mu_B(\langle n_{m\uparrow} \rangle - \langle n_{m\downarrow} \rangle + \langle n_{\bar{m}\uparrow} \rangle - \langle n_{\bar{m}\downarrow} \rangle), \tag{10}$$

and the orbital polarization per site is defined as

$$l_z = m\mu_B \left(\langle n_{m\uparrow}\rangle - \langle n_{\bar{m}\uparrow}\rangle + \langle n_{m\downarrow}\rangle - \langle n_{\bar{m}\downarrow}\rangle\right). \tag{11}$$

Introduce the particle numbers of the parallel ($n_p$) and antiparallel ($n_{ap}$) states of the spin $\sigma$ and orbital $m$:

$$\begin{aligned} n_p &= \langle n_{m\uparrow}\rangle + \langle n_{\bar{m}\downarrow}\rangle, \\ n_{ap} &= \langle n_{\bar{m}\uparrow}\rangle + \langle n_{m\downarrow}\rangle. \end{aligned} \tag{12}$$

The occupation numbers of different states can be written as

$$\begin{aligned} \langle n_{m\uparrow}\rangle &= \frac{1}{4}\left(\frac{s_z}{\mu_B} + \frac{l_z}{\mu_B m} + 2n_p\right), \\ \langle n_{\bar{m}\downarrow}\rangle &= \frac{1}{4}\left(-\frac{s_z}{\mu_B} - \frac{l_z}{\mu_B m} + 2n_p\right), \\ \langle n_{m\downarrow}\rangle &= \frac{1}{4}\left(-\frac{s_z}{\mu_B} + \frac{l_z}{\mu_B m} + 2n_{ap}\right), \\ \langle n_{\bar{m}\uparrow}\rangle &= \frac{1}{4}\left(\frac{s_z}{\mu_B} - \frac{l_z}{\mu_B m} + 2n_{ap}\right). \end{aligned} \tag{13}$$

Then the energy $\tilde{\epsilon}_{km\sigma}$ in Eq.(9) can be rewritten as

$$\begin{aligned} \tilde{\epsilon}_{km\uparrow} &= \left(\epsilon_k + \frac{1}{2}Un_{ap} + \frac{1}{2}U'n_{ap} + \frac{1}{2}U'n_p - \frac{1}{2}J_H n_{ap}\right) \\ &\quad - \mu_B\left(h + \frac{U+J_H}{4\mu_B^2}s_z\right) - \frac{1}{2}m\left(\lambda_{so} - \frac{U-2U'+J_H}{2\mu_B m^2}l_z\right), \\ \tilde{\epsilon}_{k\bar{m}\downarrow} &= \left(\epsilon_k + \frac{1}{2}Un_{ap} + \frac{1}{2}U'n_{ap} + \frac{1}{2}U'n_p - \frac{1}{2}J_H n_{ap}\right) \\ &\quad + \mu_B\left(h + \frac{U+J_H}{4\mu_B^2}s_z\right) + \frac{1}{2}m\left(-\lambda_{so} - \frac{U-2U'+J_H}{2\mu_B m^2}l_z\right), \\ \tilde{\epsilon}_{km\downarrow} &= \left(\epsilon_k + \frac{1}{2}Un_p + \frac{1}{2}U'n_p + \frac{1}{2}U'n_{ap} - \frac{1}{2}J_H n_p\right) \\ &\quad + \mu_B\left(h + \frac{U+J_H}{4\mu_B^2}s_z\right) - \frac{1}{2}m\left(-\lambda_{so} - \frac{U-2U'+J_H}{2\mu_B m^2}l_z\right), \\ \tilde{\epsilon}_{k\bar{m}\uparrow} &= \left(\epsilon_k + \frac{1}{2}Un_p + \frac{1}{2}U'n_p + \frac{1}{2}U'n_{ap} - \frac{1}{2}J_H n_p\right) \\ &\quad - \mu_B\left(h + \frac{U+J_H}{4\mu_B^2}s_z\right) + \frac{1}{2}m\left(\lambda_{so} - \frac{U-2U'+J_H}{2\mu_B m^2}l_z\right). \end{aligned} \tag{14}$$

### A. Spin Polarization without SOC

It is noted that without the external magnetic field $h$ and SOC $\lambda_{so}$, the four energy bands with spin $\sigma$ ($\uparrow$ and $\downarrow$) and orbital $m$ (for example 1 and $-1$) are degenerate, and the occupation numbers in Eq.(12) have the relation $n_{ap} = n_p$. The lattice system has the translational symmetry

$$\langle n_{m\sigma}\rangle = \frac{1}{N}\sum_i \langle n_{im\sigma}\rangle = \frac{1}{N}\sum_{\mathbf{k}} \langle n_{\mathbf{k}m\sigma}\rangle = \frac{1}{N}\sum_{\mathbf{k}} f\left(\tilde{\epsilon}_{\mathbf{k}m\sigma}\right), \tag{15}$$

where $f$ is the Fermi distribution function. Then the spin polarization in Eq.(10) can be written as

$$\begin{aligned} s_z &= \mu_B\left(\langle n_{m\uparrow}\rangle - \langle n_{m\downarrow}\rangle + \langle n_{\bar{m}\uparrow}\rangle - \langle n_{\bar{m}\downarrow}\rangle\right) \\ &= \frac{\mu_B}{N}\sum_k \left[f\left(\tilde{\epsilon}_{km\uparrow}\right) - f\left(\tilde{\epsilon}_{km\downarrow}\right) + f\left(\tilde{\epsilon}_{k\bar{m}\uparrow}\right) - f\left(\tilde{\epsilon}_{k\bar{m}\downarrow}\right)\right]. \end{aligned} \tag{16}$$

When $h=0$, the system is in a paramagnetic (PM) state. $f(\tilde{\epsilon}_{\mathbf{k}m\sigma})$ can be expanded according to $h$, which is small compared to the Fermi energy,

$$f\left(\tilde{\epsilon}_{km\sigma}\right) \approx f\left(\tilde{\epsilon}_{PM,km\sigma}\right) + \left(\tilde{\epsilon}_{km\sigma} - \tilde{\epsilon}_{PM,km\sigma}\right) \left.\frac{\partial f(E)}{\partial E}\right|_{E=\tilde{\epsilon}_{PM,km\sigma}}, \tag{17}$$

where

$$\begin{aligned}
\tilde{\epsilon}_{PM,km\uparrow} &= \left(\epsilon_k + \frac{1}{2}Un_{ap} + \frac{1}{2}U'n_{ap} + \frac{1}{2}U'n_p - \frac{1}{2}Jn_{ap}\right), \\
\tilde{\epsilon}_{PM,k\bar{m}\uparrow} &= \left(\epsilon_k + \frac{1}{2}Un_p + \frac{1}{2}U'n_p + \frac{1}{2}U'n_{ap} - \frac{1}{2}Jn_p\right), \\
\tilde{\epsilon}_{PM,km\downarrow} &= \left(\epsilon_k + \frac{1}{2}Un_p + \frac{1}{2}U'n_p + \frac{1}{2}U'n_{ap} - \frac{1}{2}Jn_p\right), \\
\tilde{\epsilon}_{PM,k\bar{m}\downarrow} &= \left(\epsilon_k + \frac{1}{2}Un_{ap} + \frac{1}{2}U'n_{ap} + \frac{1}{2}U'n_p - \frac{1}{2}Jn_{ap}\right).
\end{aligned} \tag{18}$$

When $h=0$, $n_{ap}=n_p$, it has

$$\mu_B \sum_k \left[f\left(\tilde{\epsilon}_{PM,km\uparrow}\right) - f\left(\tilde{\epsilon}_{PM,km\downarrow}\right) + f\left(\tilde{\epsilon}_{PM,k\bar{m}\uparrow}\right) - f\left(\tilde{\epsilon}_{PM,k\bar{m}\downarrow}\right)\right] = 0. \tag{19}$$

The spin polarization in Eq.(16) can be calculated up to the first order of $h$,

$$s_z \approx \left(\mu_B^2 h + \frac{U+J_H}{4}s_z\right)\int_0^\infty \left[-\frac{\partial f(E)}{\partial E}\right]\left[\rho_{m\uparrow}(E) + \rho_{\bar{m}\uparrow}(E) + \rho_{m\downarrow}(E) + \rho_{\bar{m}\downarrow}(E)\right] dE, \tag{20}$$

Then

$$s_z \approx \left(\mu_B^2 h + \frac{U+J_H}{4}s_z\right) 4\rho_0, \tag{21}$$

where

$$\rho_0 = \frac{1}{4N}\int_0^\infty \left[-\frac{\partial f(E)}{\partial E}\right]\left[\rho_{m\uparrow}(E) + \rho_{\bar{m}\uparrow}(E) + \rho_{m\downarrow}(E) + \rho_{\bar{m}\downarrow}(E)\right] dE, \tag{22}$$

which is the average density of states. Then the spin polarization per site can be calculated as

$$s_z = \frac{4\mu_B^2\rho_0}{1-(U+J_H)\rho_0}h. \tag{23}$$

The magnetic susceptibility can be written as

$$\chi = \frac{\partial s_z}{\partial h} = \frac{4\mu_B^2\rho_0}{1-(U+J_H)\rho_0} \tag{24}$$

The instability condition of the spin polarization in ferromagnets can be obtained as

$$(U+J_H)\rho_0 > 1. \tag{25}$$

### B. Spin Polarization with SOC

If we consider the SOC, the spin polarization in Eq.(16) can be calculated up to the first order of $h$ and $\lambda_{so}$.

$$\begin{aligned}
s_z \approx & \left(\mu_B^2 h + \frac{U+J_H}{4}s_z\right)\int_0^\infty \left[-\frac{\partial f(E)}{\partial E}\right]\left[\rho_{m\uparrow}(E) + \rho_{\bar{m}\uparrow}(E) + \rho_{m\downarrow}(E) + \rho_{\bar{m}\downarrow}(E)\right] dE \\
& + \frac{1}{2}\mu_B m\lambda_{so}\int_0^\infty \left[-\frac{\partial f(E)}{\partial E}\right]\left[\rho_{m\uparrow}(E) - \rho_{\bar{m}\uparrow}(E) - \rho_{m\downarrow}(E) + \rho_{\bar{m}\downarrow}(E)\right] dE.
\end{aligned} \tag{26}$$

In Eq.(26), the term proportional to the orbital polarization $l_z$ has been ignored, since $l_z$ is a small value compared to the spin polarization $s_z$. Then, it has

$$s_z \approx \left(\mu_B^2 h + \frac{U+J_H}{4} s_z\right) 4\rho_0 + m\mu_B \lambda_{so} \rho_{p-ap}, \tag{27}$$

where

$$\rho_{p-ap} = \frac{1}{2}\int_0^\infty \left[-\frac{\partial f(E)}{\partial E}\right] \left[\rho_{m\uparrow}(E) + \rho_{\bar{m}\downarrow}(E) - \rho_{\bar{m}\uparrow}(E) - \rho_{m\downarrow}(E)\right] dE, \tag{28}$$

which is the difference of the density of sates with parallel spin $\sigma$ and orbital $m$ and that with antiparallel $\sigma$ and $m$. Then the spin polarization per site can be calculated as

$$s_z = \frac{4\mu_B^2 \rho_0 h + m\mu_B \lambda_{so} \rho_{p-ap}}{1-(U+J_H)\rho_0}. \tag{29}$$

The magnetic susceptibility $\chi$ is the same as in Eq. (24), and the instability condition of the spin polarization with SOC is the same as that without SOC in Eq. (25).

### C. Orbital Polarization from SOC

Similarly, by Eq.(15) the orbital polarization in Eq.(11) can be expressed as

$$\begin{aligned} l_z &= m\mu_B \left(\langle n_{m\uparrow}\rangle - \langle n_{\bar{m}\uparrow}\rangle + \langle n_{m\downarrow}\rangle - \langle n_{\bar{m}\downarrow}\rangle\right) \\ &= \frac{m\mu_B}{N}\sum_k \left[f\left(\tilde{\epsilon}_{km\uparrow}\right) - f\left(\tilde{\epsilon}_{k\bar{m}\uparrow}\right) + f\left(\tilde{\epsilon}_{km\downarrow}\right) - f\left(\tilde{\epsilon}_{k\bar{m}\downarrow}\right)\right]. \end{aligned} \tag{30}$$

On the basis of ferromagnetic (FM) state, the SOC can be regarded as a value, which is small compared to the Fermi energy[1], so $f(\tilde{\epsilon}_{\mathbf{k}m\sigma})$ can be expanded according to $\lambda_{so}$

$$f\left(\tilde{\epsilon}_{km\sigma}\right) \approx f\left(\tilde{\epsilon}_{FM,km\sigma}\right) + \left[\frac{\partial f(E)}{\partial E}\right]_{E=\tilde{\epsilon}_{FM,km\sigma}} \left(\tilde{\epsilon}_{km\sigma} - \tilde{\epsilon}_{FM,km\sigma}\right), \tag{31}$$

where

$$\begin{aligned} \tilde{\epsilon}_{FM,km\uparrow} &= \left(\epsilon_k + \frac{1}{2}Un_{ap} + \frac{1}{2}U'n_{ap} + \frac{1}{2}U'n_p - \frac{1}{2}J_H n_{ap}\right) - \mu_B\left(h + \frac{U+J_H}{4\mu_B^2}s_z\right), \\ \tilde{\epsilon}_{FM,k\bar{m}\uparrow} &= \left(\epsilon_k + \frac{1}{2}Un_p + \frac{1}{2}U'n_p + \frac{1}{2}U'n_{ap} - \frac{1}{2}J_H n_p\right) - \mu_B\left(h + \frac{U+J_H}{4\mu_B^2}s_z\right), \\ \tilde{\epsilon}_{FM,km\downarrow} &= \left(\epsilon_k + \frac{1}{2}Un_p + \frac{1}{2}U'n_p + \frac{1}{2}U'n_{ap} - \frac{1}{2}J_H n_p\right) + \mu_B\left(h + \frac{U+J_H}{4\mu_B^2}s_z\right), \\ \tilde{\epsilon}_{FM,k\bar{m}\downarrow} &= \left(\epsilon_k + \frac{1}{2}Un_{ap} + \frac{1}{2}U'n_{ap} + \frac{1}{2}U'n_p - \frac{1}{2}J_H n_{ap}\right) + \mu_B\left(h + \frac{U+J_H}{4\mu_B^2}s_z\right). \end{aligned} \tag{32}$$

By Eq.(14) it yields

$$\tilde{\epsilon}_{km\sigma} - \tilde{\epsilon}_{FM,km\sigma} = -\frac{1}{2}m\left(\sigma\lambda_{so} - \frac{U-2U'+J_H}{2\mu_B m^2}l_z\right). \tag{33}$$

When $\lambda_{so}=0$, $n_{ap}=n_p$, we have

$$\frac{m\mu_B}{N}\sum_k \left[f\left(\tilde{\epsilon}_{FM,km\uparrow}\right) - f\left(\tilde{\epsilon}_{FM,k\bar{m}\uparrow}\right) + f\left(\tilde{\epsilon}_{FM,km\downarrow}\right) - f\left(\tilde{\epsilon}_{FM,k\bar{m}\downarrow}\right)\right] = 0. \tag{34}$$

The orbital polarization in Eq.(30) can be calculated up to the first order of $\lambda_{so}$,

$$\begin{aligned} l_z \approx{}& \frac{1}{2}m^2\mu_B\lambda_{so}\int_0^\infty \left[-\frac{\partial f(E)}{\partial E}\right]\left[\rho_{m\uparrow}(E) + \rho_{\bar{m}\uparrow}(E) - \rho_{m\downarrow}(E) - \rho_{\bar{m}\downarrow}(E)\right] dE \\ &+ \frac{1}{4}\left(2U'-U-J_H\right)l_z\int_0^\infty \left[-\frac{\partial f(E)}{\partial E}\right]\left[\rho_{m\uparrow}(E) + \rho_{\bar{m}\uparrow}(E) + \rho_{m\downarrow}(E) + \rho_{\bar{m}\downarrow}(E)\right] dE. \end{aligned} \tag{35}$$

Then

$$l_z \approx m^2\mu_B\lambda_{so}\rho_s + (2U' - U - J_H)\,\rho_0 l_z, \tag{36}$$

where

$$\rho_s = \frac{1}{2N}\int_0^\infty \left[-\frac{\partial f(E)}{\partial E}\right]\left[\rho_{m\uparrow}(E) + \rho_{\bar{m}\uparrow}(E) - \rho_{m\downarrow}(E) - \rho_{\bar{m}\downarrow}(E)\right] dE, \tag{37}$$

which is the average spin polarized density of states. Thus, the orbital polarization per site can be calculated as

$$l_z = \frac{m^2\mu_B\rho_s}{1 - (2U' - U - J_H)\,\rho_0}\lambda_{so}, \tag{38}$$

where $\rho_0$ is given by Eq.(22). And Eq.(38) can be rewritten as

$$l_z = \mu_B m^2 \rho_s \lambda_{so}^{\text{eff}}, \tag{39}$$

where the effective SOC $\lambda_{so}^{\text{eff}}$ is expressed as

$$\lambda_{so}^{\text{eff}} = \frac{\lambda_{so}}{1 - (2U' - U - J_H)\,\rho_0}. \tag{40}$$

The instability condition of orbital polarization from SOC in ferromagnets can be obtained as

$$(2U' - U - J_H)\rho_0 > 1. \tag{41}$$

## II. FIVE-ORBITAL HUBBARD MODEL WITH SOC

As an extension of the above two-orbital model, in this section we consider the five-orbital Hubbard model with the SOC. The Hamiltonian is written as

$$H = \sum_{\mathbf{k},m,\sigma} \epsilon_{\mathbf{k}m\sigma} n_{\mathbf{k}m\sigma} + U\sum_{i,m} n_{im\uparrow}n_{im\downarrow} + \frac{U'}{2}\sum_{i,m\neq m',\sigma,\sigma'} n_{im\sigma}n_{im'\sigma'} - \frac{J_H}{2}\sum_{i,m\neq m',\sigma} n_{im\sigma}n_{im'\sigma}, \tag{42}$$

where $\epsilon_{\mathbf{k}m\sigma}$ is the energy for electron with wave vector $\mathbf{k}$, orbital $m$ ($m$ = 2, 1, 0, -1, -2 for the transition metals), and spin $\sigma$ $(\uparrow, \downarrow)$, $U$ is the on-site Coulomb repulsion within the orbital $m$, $U'$ is the on-site Coulomb repulsion between different orbitals $m$ and $m'$, and $J_H$ is the Hund coupling. $n_{\mathbf{k}m\sigma}(n_{im\sigma})$ represents the particle number of electron with wave vector $\mathbf{k}$ (site index $i$), orbital $m$ and spin $\sigma$. For simplicity, we consider five degenerate energy bands, which are lifted by external magnetic field $h$ and the Ising-type SOC[1]

$$\epsilon_{\mathbf{k}m\sigma} = \epsilon_{\mathbf{k}} - \sigma\mu_B h - \frac{1}{2}\sigma\lambda_{so}m, \tag{43}$$

where $\lambda_{so}$ is the SOC constant, $\epsilon_{\mathbf{k}}$ is the electron energy without the external magnetic filed and SOC. Using the Hartree-Fock approximation

$$n_{im\sigma}n_{im'\sigma'} \approx \langle n_{im\sigma}\rangle\, n_{im'\sigma'} + \langle n_{im'\sigma'}\rangle\, n_{im\sigma} - \langle n_{im\sigma}\rangle \langle n_{im'\sigma'}\rangle\,, \tag{44}$$

the interaction terms can be written separately as:

$$
\begin{aligned}
n_{i\bar{2}\uparrow}n_{i\bar{2}\downarrow} &= n_{i\bar{2}\downarrow}n_{i\bar{2}\uparrow} \approx \langle n_{i\bar{2}\downarrow} \rangle n_{i\bar{2}\uparrow} + \langle n_{i\bar{2}\uparrow} \rangle n_{i\bar{2}\downarrow} - \langle n_{i\bar{2}\uparrow} \rangle \langle n_{i\bar{2}\downarrow} \rangle , \\
n_{i\bar{1}\uparrow}n_{i\bar{1}\downarrow} &= n_{l\bar{1}\downarrow}n_{i\bar{1}\uparrow} \approx \langle n_{i\bar{1}\downarrow} \rangle n_{i\bar{1}\uparrow} + \langle n_{i\bar{1}\uparrow} \rangle n_{i\bar{1}\downarrow} - \langle n_{i\bar{1}\uparrow} \rangle \langle n_{i\bar{1}\downarrow} \rangle , \\
n_{i0\uparrow}n_{i0\downarrow} &= n_{i0\downarrow}n_{i0\uparrow} \approx \langle n_{i0\downarrow} \rangle n_{i0\uparrow} + \langle n_{i0\uparrow} \rangle n_{i0\downarrow} - \langle n_{i0\uparrow} \rangle \langle n_{i0\downarrow} \rangle , \\
n_{i1\uparrow}n_{i1\downarrow} &= n_{i1\downarrow}n_{i1\uparrow} \approx \langle n_{i1\downarrow} \rangle n_{i1\uparrow} + \langle n_{i1\uparrow} \rangle n_{i1\downarrow} - \langle n_{i1\uparrow} \rangle \langle n_{i1\downarrow} \rangle , \\
n_{i2\uparrow}n_{i2\downarrow} &= n_{i2\downarrow}n_{i2\uparrow} \approx \langle n_{i2\downarrow} \rangle n_{i2\uparrow} + \langle n_{i2\uparrow} \rangle n_{i2\downarrow} - \langle n_{i2\uparrow} \rangle \langle n_{i2\downarrow} \rangle , \\
n_{i1\uparrow}n_{i\bar{2}\uparrow} &= n_{i\bar{2}\uparrow}n_{i1\uparrow} \approx \langle n_{i1\uparrow} \rangle n_{i\bar{2}\uparrow} + \langle n_{i\bar{2}\uparrow} \rangle n_{i1\uparrow} - \langle n_{i1\uparrow} \rangle \langle n_{i\bar{2}\uparrow} \rangle , \\
n_{i1\downarrow}n_{i\bar{2}\downarrow} &= n_{i\bar{2}\downarrow}n_{i1\downarrow} \approx \langle n_{i1\downarrow} \rangle n_{i\bar{2}\downarrow} + \langle n_{i\bar{2}\downarrow} \rangle n_{i1\downarrow} - \langle n_{i1\downarrow} \rangle \langle n_{i\bar{2}\downarrow} \rangle , \\
n_{i1\uparrow}n_{i\bar{2}\downarrow} &= n_{i\bar{2}\uparrow}n_{i1\downarrow} \approx \langle n_{i1\uparrow} \rangle n_{i\bar{2}\downarrow} + \langle n_{i\bar{2}\uparrow} \rangle n_{i1\downarrow} - \langle n_{i1\uparrow} \rangle \langle n_{i\bar{2}\downarrow} \rangle , \\
n_{i1\downarrow}n_{i\bar{2}\uparrow} &= n_{i\bar{2}\downarrow}n_{i1\uparrow} \approx \langle n_{i1\downarrow} \rangle n_{i\bar{2}\uparrow} + \langle n_{i\bar{2}\downarrow} \rangle n_{i1\uparrow} - \langle n_{i1\downarrow} \rangle \langle n_{i\bar{2}\uparrow} \rangle , \\
n_{i1\uparrow}n_{i\bar{1}\uparrow} &= n_{i\bar{1}\uparrow}n_{i1\uparrow} \approx \langle n_{i1\uparrow} \rangle n_{i\bar{1}\uparrow} + \langle n_{i\bar{1}\uparrow} \rangle n_{i1\uparrow} - \langle n_{i1\uparrow} \rangle \langle n_{i\bar{1}\uparrow} \rangle , \\
n_{i1\downarrow}n_{i\bar{1}\downarrow} &= n_{i\bar{1}\downarrow}n_{i1\downarrow} \approx \langle n_{i1\downarrow} \rangle n_{i\bar{1}\downarrow} + \langle n_{i\bar{1}\downarrow} \rangle n_{i1\downarrow} - \langle n_{i1\downarrow} \rangle \langle n_{i\bar{1}\downarrow} \rangle , \\
n_{i1\uparrow}n_{i\bar{1}\downarrow} &= n_{i\bar{1}\uparrow}n_{i1\downarrow} \approx \langle n_{i1\uparrow} \rangle n_{i\bar{1}\downarrow} + \langle n_{i\bar{1}\uparrow} \rangle n_{i1\downarrow} - \langle n_{i1\uparrow} \rangle \langle n_{i\bar{1}\downarrow} \rangle , \\
n_{i1\downarrow}n_{i\bar{1}\uparrow} &= n_{i\bar{1}\downarrow}n_{i1\uparrow} \approx \langle n_{i1\downarrow} \rangle n_{i\bar{1}\uparrow} + \langle n_{i\bar{1}\downarrow} \rangle n_{i1\uparrow} - \langle n_{i1\downarrow} \rangle \langle n_{i\bar{1}\uparrow} \rangle , \\
n_{i1\uparrow}n_{i0\uparrow} &= n_{i0\uparrow}n_{i1\uparrow} \approx \langle n_{i1\uparrow} \rangle n_{i0\uparrow} + \langle n_{i0\uparrow} \rangle n_{i1\uparrow} - \langle n_{i1\uparrow} \rangle \langle n_{i0\uparrow} \rangle , \\
n_{i1\downarrow}n_{i0\downarrow} &= n_{i0\downarrow}n_{i1\downarrow} \approx \langle n_{i1\downarrow} \rangle n_{i0\downarrow} + \langle n_{i0\downarrow} \rangle n_{i1\downarrow} - \langle n_{i1\downarrow} \rangle \langle n_{i0\downarrow} \rangle , \\
n_{i1\uparrow}n_{i0\downarrow} &= n_{i0\uparrow}n_{i1\downarrow} \approx \langle n_{i1\uparrow} \rangle n_{i0\downarrow} + \langle n_{i0\uparrow} \rangle n_{i1\downarrow} - \langle n_{i1\uparrow} \rangle \langle n_{i0\downarrow} \rangle , \\
n_{i1\downarrow}n_{i0\uparrow} &= n_{i0\downarrow}n_{i1\uparrow} \approx \langle n_{i1\downarrow} \rangle n_{i0\uparrow} + \langle n_{i0\downarrow} \rangle n_{i1\uparrow} - \langle n_{i1\downarrow} \rangle \langle n_{i0\uparrow} \rangle , \\
n_{i1\uparrow}n_{i2\uparrow} &= n_{i2\uparrow}n_{i1\uparrow} \approx \langle n_{i1\uparrow} \rangle n_{i2\uparrow} + \langle n_{i2\uparrow} \rangle n_{i1\uparrow} - \langle n_{i1\uparrow} \rangle \langle n_{i2\uparrow} \rangle , \\
n_{i1\downarrow}n_{i2\downarrow} &= n_{i2\downarrow}n_{i1\downarrow} \approx \langle n_{i1\downarrow} \rangle n_{i2\downarrow} + \langle n_{i2\downarrow} \rangle n_{i1\downarrow} - \langle n_{i1\downarrow} \rangle \langle n_{i2\downarrow} \rangle , \\
n_{i1\uparrow}n_{i2\downarrow} &= n_{i2\uparrow}n_{i1\downarrow} \approx \langle n_{i1\uparrow} \rangle n_{i2\downarrow} + \langle n_{i2\uparrow} \rangle n_{i1\downarrow} - \langle n_{i1\uparrow} \rangle \langle n_{i2\downarrow} \rangle , \\
n_{i1\downarrow}n_{i2\uparrow} &= n_{i2\downarrow}n_{i1\uparrow} \approx \langle n_{i1\downarrow} \rangle n_{i2\uparrow} + \langle n_{i2\downarrow} \rangle n_{i1\uparrow} - \langle n_{i1\downarrow} \rangle \langle n_{i2\uparrow} \rangle , \\
n_{i2\uparrow}n_{i\bar{2}\uparrow} &= n_{i\bar{2}\uparrow}n_{i2\uparrow} \approx \langle n_{i2\uparrow} \rangle n_{i\bar{2}\uparrow} + \langle n_{i\bar{2}\uparrow} \rangle n_{i2\uparrow} - \langle n_{i2\uparrow} \rangle \langle n_{i\bar{2}\uparrow} \rangle , \\
n_{i2\downarrow}n_{i\bar{2}\downarrow} &= n_{i\bar{2}\downarrow}n_{i2\downarrow} \approx \langle n_{i2\downarrow} \rangle n_{i\bar{2}\downarrow} + \langle n_{i\bar{2}\downarrow} \rangle n_{i2\downarrow} - \langle n_{i2\downarrow} \rangle \langle n_{i\bar{2}\downarrow} \rangle , \\
n_{i2\uparrow}n_{i\bar{2}\downarrow} &= n_{i\bar{2}\uparrow}n_{i2\downarrow} \approx \langle n_{i2\uparrow} \rangle n_{i\bar{2}\downarrow} + \langle n_{i\bar{2}\uparrow} \rangle n_{i2\downarrow} - \langle n_{i2\uparrow} \rangle \langle n_{i\bar{2}\downarrow} \rangle , \\
n_{i2\downarrow}n_{i\bar{2}\uparrow} &= n_{i\bar{2}\downarrow}n_{i2\uparrow} \approx \langle n_{i2\downarrow} \rangle n_{i\bar{2}\uparrow} + \langle n_{i\bar{2}\downarrow} \rangle n_{i2\uparrow} - \langle n_{i2\downarrow} \rangle \langle n_{i\bar{2}\uparrow} \rangle , \\
n_{i2\uparrow}n_{i\bar{1}\uparrow} &= n_{i\bar{1}\uparrow}n_{i2\uparrow} \approx \langle n_{i2\uparrow} \rangle n_{i\bar{1}\uparrow} + \langle n_{i\bar{1}\uparrow} \rangle n_{i2\uparrow} - \langle n_{i2\uparrow} \rangle \langle n_{i\bar{1}\uparrow} \rangle , \\
n_{i2\downarrow}n_{i\bar{1}\downarrow} &= n_{i\bar{1}\downarrow}n_{i2\downarrow} \approx \langle n_{i2\downarrow} \rangle n_{i\bar{1}\downarrow} + \langle n_{i\bar{1}\downarrow} \rangle n_{i2\downarrow} - \langle n_{i2\downarrow} \rangle \langle n_{i\bar{1}\downarrow} \rangle , \\
n_{i2\uparrow}n_{i\bar{1}\downarrow} &= n_{i\bar{1}\uparrow}n_{i2\downarrow} \approx \langle n_{i2\uparrow} \rangle n_{i\bar{1}\downarrow} + \langle n_{i\bar{1}\uparrow} \rangle n_{i2\downarrow} - \langle n_{i2\uparrow} \rangle \langle n_{i\bar{1}\downarrow} \rangle , \\
n_{i2\downarrow}n_{i\bar{1}\uparrow} &= n_{i\bar{1}\downarrow}n_{i2\uparrow} \approx \langle n_{i2\downarrow} \rangle n_{i\bar{1}\uparrow} + \langle n_{i\bar{1}\downarrow} \rangle n_{i2\uparrow} - \langle n_{i2\downarrow} \rangle \langle n_{i\bar{1}\uparrow} \rangle , \\
n_{i2\uparrow}n_{i0\uparrow} &= n_{i0\uparrow}n_{i2\uparrow} \approx \langle n_{i2\uparrow} \rangle n_{i0\uparrow} + \langle n_{i0\uparrow} \rangle n_{i2\uparrow} - \langle n_{i2\uparrow} \rangle \langle n_{l0\uparrow} \rangle , \\
n_{i2\downarrow}n_{i0\downarrow} &= n_{i0\downarrow}n_{i2\downarrow} \approx \langle n_{i2\downarrow} \rangle n_{i0\downarrow} + \langle n_{i0\downarrow} \rangle n_{i2\downarrow} - \langle n_{i2\downarrow} \rangle \langle n_{i0\downarrow} \rangle , \\
n_{i2\uparrow}n_{i0\downarrow} &= n_{i0\uparrow}n_{i2\downarrow} \approx \langle n_{i2\uparrow} \rangle n_{i0\downarrow} + \langle n_{i0\uparrow} \rangle n_{i2\downarrow} - \langle n_{i2\uparrow} \rangle \langle n_{i0\downarrow} \rangle , \\
n_{i2\downarrow}n_{i0\uparrow} &= n_{i0\downarrow}n_{i2\uparrow} \approx \langle n_{i2\downarrow} \rangle n_{i0\uparrow} + \langle n_{i0\downarrow} \rangle n_{i2\uparrow} - \langle n_{i2\downarrow} \rangle \langle n_{i0\uparrow} \rangle , \\
n_{i0\uparrow}n_{i\bar{1}\uparrow} &= n_{i\bar{1}\uparrow}n_{i0\uparrow} \approx \langle n_{i0\uparrow} \rangle n_{i\bar{1}\uparrow} + \langle n_{i\bar{1}\uparrow} \rangle n_{i0\uparrow} - \langle n_{i0\uparrow} \rangle \langle n_{i\bar{1}\uparrow} \rangle , \\
n_{i0\downarrow}n_{i\bar{1}\downarrow} &= n_{i\bar{1}\downarrow}n_{i0\downarrow} \approx \langle n_{i0\downarrow} \rangle n_{i\bar{1}\downarrow} + \langle n_{i\bar{1}\downarrow} \rangle n_{i0\downarrow} - \langle n_{i0\downarrow} \rangle \langle n_{i\bar{1}\downarrow} \rangle , \\
n_{i0\uparrow}n_{i\bar{1}\downarrow} &= n_{i\bar{1}\uparrow}n_{i0\downarrow} \approx \langle n_{i0\uparrow} \rangle n_{i\bar{1}\downarrow} + \langle n_{i\bar{1}\uparrow} \rangle n_{i0\downarrow} - \langle n_{i0\uparrow} \rangle \langle n_{i\bar{1}\downarrow} \rangle , \\
n_{i0\downarrow}n_{i\bar{1}\uparrow} &= n_{i\bar{1}\downarrow}n_{i0\uparrow} \approx \langle n_{i0\downarrow} \rangle n_{i\bar{1}\uparrow} + \langle n_{i\bar{1}\downarrow} \rangle n_{i0\uparrow} - \langle n_{i0\downarrow} \rangle \langle n_{i\bar{1}\uparrow} \rangle , \\
n_{i0\uparrow}n_{i\bar{2}\uparrow} &= n_{i\bar{2}\uparrow}n_{i0\uparrow} \approx \langle n_{i0\uparrow} \rangle n_{i\bar{2}\uparrow} + \langle n_{i\bar{2}\uparrow} \rangle n_{i0\uparrow} - \langle n_{i0\uparrow} \rangle \langle n_{i\bar{2}\uparrow} \rangle , \\
n_{i0\downarrow}n_{i\bar{2}\downarrow} &= n_{i\bar{2}\downarrow}n_{i0\downarrow} \approx \langle n_{i0\downarrow} \rangle n_{i\bar{2}\downarrow} + \langle n_{i\bar{2}\downarrow} \rangle n_{i0\downarrow} - \langle n_{i0\downarrow} \rangle \langle n_{i\bar{2}\downarrow} \rangle , \\
n_{i0\uparrow}n_{i\bar{2}\downarrow} &= n_{i\bar{2}\uparrow}n_{i0\downarrow} \approx \langle n_{i0\uparrow} \rangle n_{i\bar{2}\downarrow} + \langle n_{i\bar{2}\uparrow} \rangle n_{i0\downarrow} - \langle n_{i0\uparrow} \rangle \langle n_{i\bar{2}\downarrow} \rangle , \\
n_{i0\downarrow}n_{i\bar{2}\uparrow} &= n_{i\bar{2}\downarrow}n_{i0\uparrow} \approx \langle n_{i0\downarrow} \rangle n_{i\bar{2}\uparrow} + \langle n_{i\bar{2}\downarrow} \rangle n_{i0\uparrow} - \langle n_{i0\downarrow} \rangle \langle n_{i\bar{2}\uparrow} \rangle , \\
n_{i\bar{1}\uparrow}n_{i\bar{2}\uparrow} &= n_{i\bar{2}\uparrow}n_{i\bar{1}\uparrow} \approx \langle n_{i\bar{1}\uparrow} \rangle n_{i\bar{2}\uparrow} + \langle n_{i\bar{2}\uparrow} \rangle n_{i\bar{1}\uparrow} - \langle n_{i\bar{1}\uparrow} \rangle \langle n_{i\bar{2}\uparrow} \rangle , \\
n_{i\bar{1}\downarrow}n_{i\bar{2}\downarrow} &= n_{i\bar{2}\downarrow}n_{i\bar{1}\downarrow} \approx \langle n_{i\bar{1}\downarrow} \rangle n_{i\bar{2}\downarrow} + \langle n_{i\bar{2}\downarrow} \rangle n_{i\bar{1}\downarrow} - \langle n_{i\bar{1}\downarrow} \rangle \langle n_{i\bar{2}\downarrow} \rangle , \\
n_{i\bar{1}\uparrow}n_{i\bar{2}\downarrow} &= n_{i\bar{2}\uparrow}n_{i\bar{1}\downarrow} \approx \langle n_{i\bar{1}\uparrow} \rangle n_{i\bar{2}\downarrow} + \langle n_{i\bar{2}\uparrow} \rangle n_{i\bar{1}\downarrow} - \langle n_{i\bar{1}\uparrow} \rangle \langle n_{i\bar{2}\downarrow} \rangle , \\
n_{i\bar{1}\downarrow}n_{i\bar{2}\uparrow} &= n_{i\bar{2}\downarrow}n_{i\bar{1}\uparrow} \approx \langle n_{i\bar{1}\downarrow} \rangle n_{i\bar{2}\uparrow} + \langle n_{i\bar{2}\downarrow} \rangle n_{i\bar{1}\uparrow} - \langle n_{i\bar{1}\downarrow} \rangle \langle n_{i\bar{2}\uparrow} \rangle .
\end{aligned}
\tag{45}
$$

Assuming the system is uniform, and the occupation number $n_{im\sigma}$ is independent of lattice site $i$,

$$\langle n_{im\sigma}\rangle \approx \langle n_{m\sigma}\rangle\,, \tag{46}$$

and making the Fourier transformation:

$$\sum_i n_{im\sigma} = \sum_{\mathbf{k}} n_{\mathbf{k}m\sigma}, \tag{47}$$

the Hamiltonian in Eq.(42) can be diagonalized as

$$H \approx \sum_{\mathbf{k},m,\sigma} \tilde{\epsilon}_{\mathbf{k}m\sigma} n_{\mathbf{k}m\sigma}, \tag{48}$$

with

$$\begin{aligned}
\tilde{\epsilon}_{k\bar{2}\uparrow} =& \epsilon_k - \mu_B h + \lambda + U\left\langle n_{\bar{2}\downarrow}\right\rangle \\
&+ U'\left(\left\langle n_{1\uparrow}\right\rangle + \left\langle n_{1\downarrow}\right\rangle + \left\langle n_{2\uparrow}\right\rangle + \left\langle n_{2\downarrow}\right\rangle + \left\langle n_{0\uparrow}\right\rangle + \left\langle n_{0\downarrow}\right\rangle + \left\langle n_{\bar{1}\uparrow}\right\rangle + \left\langle n_{\bar{1}\downarrow}\right\rangle\right) \\
&- J_H\left(\left\langle n_{1\uparrow}\right\rangle + \left\langle n_{2\uparrow}\right\rangle + \left\langle n_{0\uparrow}\right\rangle + \left\langle n_{\bar{1}\uparrow}\right\rangle\right), \\
\tilde{\epsilon}_{k\bar{1}\uparrow} =& \epsilon_k - \mu_B h + \frac{1}{2}\lambda + U\left\langle n_{\bar{1}\downarrow}\right\rangle \\
&+ U'\left(\left\langle n_{1\uparrow}\right\rangle + \left\langle n_{1\downarrow}\right\rangle + \left\langle n_{2\uparrow}\right\rangle + \left\langle n_{2\downarrow}\right\rangle + \left\langle n_{0\uparrow}\right\rangle + \left\langle n_{0\downarrow}\right\rangle + \left\langle n_{\bar{2}\uparrow}\right\rangle + \left\langle n_{\bar{2}\downarrow}\right\rangle\right) \\
&- J_H\left(\left\langle n_{1\uparrow}\right\rangle + \left\langle n_{2\uparrow}\right\rangle + \left\langle n_{0\uparrow}\right\rangle + \left\langle n_{\bar{2}\uparrow}\right\rangle\right), \\
\tilde{\epsilon}_{k0\uparrow} =& \epsilon_k - \mu_B h + U\left\langle n_{0\downarrow}\right\rangle \\
&+ U'\left(\left\langle n_{1\uparrow}\right\rangle + \left\langle n_{1\downarrow}\right\rangle + \left\langle n_{2\uparrow}\right\rangle + \left\langle n_{2\downarrow}\right\rangle + \left\langle n_{\bar{1}\uparrow}\right\rangle + \left\langle n_{\bar{1}\downarrow}\right\rangle + \left\langle n_{\bar{2}\uparrow}\right\rangle + \left\langle n_{\bar{2}\downarrow}\right\rangle\right) \\
&- J_H\left(\left\langle n_{1\uparrow}\right\rangle + \left\langle n_{2\uparrow}\right\rangle + \left\langle n_{\bar{1}\uparrow}\right\rangle + \left\langle n_{\bar{2}\uparrow}\right\rangle\right), \\
\tilde{\epsilon}_{k1\uparrow} =& \epsilon_k - \mu_B h - \frac{1}{2}\lambda + U\left\langle n_{1\downarrow}\right\rangle \\
&+ U'\left(\left\langle n_{2\uparrow}\right\rangle + \left\langle n_{2\downarrow}\right\rangle + \left\langle n_{0\uparrow}\right\rangle + \left\langle n_{0\downarrow}\right\rangle + \left\langle n_{\bar{1}\uparrow}\right\rangle + \left\langle n_{\bar{1}\downarrow}\right\rangle + \left\langle n_{\bar{2}\uparrow}\right\rangle + \left\langle n_{\bar{2}\downarrow}\right\rangle\right) \\
&- J_H\left(\left\langle n_{2\uparrow}\right\rangle + \left\langle n_{0\uparrow}\right\rangle + \left\langle n_{\bar{1}\uparrow}\right\rangle + \left\langle n_{\bar{2}\uparrow}\right\rangle\right), \\
\tilde{\epsilon}_{k2\uparrow} =& \epsilon_k - \mu_B h - \lambda + U\left\langle n_{2\downarrow}\right\rangle \\
&+ U'\left(\left\langle n_{1\uparrow}\right\rangle + \left\langle n_{1\downarrow}\right\rangle + \left\langle n_{0\uparrow}\right\rangle + \left\langle n_{0\downarrow}\right\rangle + \left\langle n_{\bar{1}\uparrow}\right\rangle + \left\langle n_{\bar{1}\downarrow}\right\rangle + \left\langle n_{\bar{2}\uparrow}\right\rangle + \left\langle n_{\bar{2}\downarrow}\right\rangle\right) \\
&- J_H\left(\left\langle n_{1\uparrow}\right\rangle + \left\langle n_{0\uparrow}\right\rangle + \left\langle n_{\bar{1}\uparrow}\right\rangle + \left\langle n_{\bar{2}\uparrow}\right\rangle\right), \\
\tilde{\epsilon}_{k\bar{2}\downarrow} =& \epsilon_k - \mu_B h - \lambda + U\left\langle n_{\bar{2}\uparrow}\right\rangle \\
&+ U'\left(\left\langle n_{1\uparrow}\right\rangle + \left\langle n_{1\downarrow}\right\rangle + \left\langle n_{2\uparrow}\right\rangle + \left\langle n_{2\downarrow}\right\rangle + \left\langle n_{0\uparrow}\right\rangle + \left\langle n_{0\downarrow}\right\rangle + \left\langle n_{\bar{1}\uparrow}\right\rangle + \left\langle n_{\bar{1}\downarrow}\right\rangle\right) \\
&- J_H\left(\left\langle n_{1\downarrow}\right\rangle + \left\langle n_{2\downarrow}\right\rangle + \left\langle n_{0\downarrow}\right\rangle + \left\langle n_{\bar{1}\downarrow}\right\rangle\right), \\
\tilde{\epsilon}_{k\bar{1}\downarrow} =& \epsilon_k + \mu_B h - \frac{1}{2}\lambda + U\left\langle n_{\bar{1}\uparrow}\right\rangle \\
&+ U'\left(\left\langle n_{1\uparrow}\right\rangle + \left\langle n_{1\downarrow}\right\rangle + \left\langle n_{2\uparrow}\right\rangle + \left\langle n_{2\downarrow}\right\rangle + \left\langle n_{0\uparrow}\right\rangle + \left\langle n_{0\downarrow}\right\rangle + \left\langle n_{\bar{2}\uparrow}\right\rangle + \left\langle n_{\bar{2}\downarrow}\right\rangle\right) \\
&- J_H\left(\left\langle n_{1\downarrow}\right\rangle + \left\langle n_{2\downarrow}\right\rangle + \left\langle n_{0\downarrow}\right\rangle + \left\langle n_{\bar{2}\downarrow}\right\rangle\right), \\
\tilde{\epsilon}_{k0\downarrow} =& \epsilon_k + \mu_B h + U\left\langle n_{0\uparrow}\right\rangle \\
&+ U'\left(\left\langle n_{1\uparrow}\right\rangle + \left\langle n_{1\downarrow}\right\rangle + \left\langle n_{2\uparrow}\right\rangle + \left\langle n_{2\downarrow}\right\rangle + \left\langle n_{\bar{1}\uparrow}\right\rangle + \left\langle n_{\bar{1}\downarrow}\right\rangle + \left\langle n_{\bar{2}\uparrow}\right\rangle + \left\langle n_{\bar{2}\downarrow}\right\rangle\right) \\
&- J_H\left(\left\langle n_{1\downarrow}\right\rangle + \left\langle n_{2\downarrow}\right\rangle + \left\langle n_{\bar{1}\downarrow}\right\rangle + \left\langle n_{\bar{2}\downarrow}\right\rangle\right), \\
\tilde{\epsilon}_{k\bar{1}\downarrow} =& \epsilon_k + \mu_B h + \frac{1}{2}\lambda + U\left\langle n_{1\uparrow}\right\rangle \\
&+ U'\left(\left\langle n_{2\uparrow}\right\rangle + \left\langle n_{2\downarrow}\right\rangle + \left\langle n_{0\uparrow}\right\rangle + \left\langle n_{0\downarrow}\right\rangle + \left\langle n_{\bar{1}\uparrow}\right\rangle + \left\langle n_{\bar{1}\downarrow}\right\rangle + \left\langle n_{\bar{2}\uparrow}\right\rangle + \left\langle n_{\bar{2}\downarrow}\right\rangle\right) \\
&- J_H\left(\left\langle n_{2\downarrow}\right\rangle + \left\langle n_{0\downarrow}\right\rangle + \left\langle n_{\bar{1}\downarrow}\right\rangle + \left\langle n_{\bar{2}\downarrow}\right\rangle\right), \\
\tilde{\epsilon}_{k2\downarrow} =& \epsilon_k + \mu_B h + \lambda + U\left\langle n_{2\uparrow}\right\rangle \\
&+ U'\left(\left\langle n_{1\uparrow}\right\rangle + \left\langle n_{1\downarrow}\right\rangle + \left\langle n_{0\uparrow}\right\rangle + \left\langle n_{0\downarrow}\right\rangle + \left\langle n_{\bar{1}\uparrow}\right\rangle + \left\langle n_{\bar{1}\downarrow}\right\rangle + \left\langle n_{\bar{2}\uparrow}\right\rangle + \left\langle n_{\bar{2}\downarrow}\right\rangle\right) \\
&- J_H\left(\left\langle n_{1\downarrow}\right\rangle + \left\langle n_{0\downarrow}\right\rangle + \left\langle n_{\bar{1}\downarrow}\right\rangle + \left\langle n_{\bar{2}\downarrow}\right\rangle\right).
\end{aligned} \tag{49}$$

The spin polarization per site is defined as

$$\begin{aligned}
s_z &= s_{z0} + s_{z1} + s_{z2}, \\
s_{z0} &= \mu_B(\langle n_{0\uparrow}\rangle - \langle n_{0\downarrow}\rangle), \\
s_{z1} &= \mu_B(\langle n_{1\uparrow}\rangle - \langle n_{1\downarrow}\rangle + \langle n_{\bar{1}\uparrow}\rangle - \langle n_{\bar{1}\downarrow}\rangle), \\
s_{z2} &= \mu_B(\langle n_{2\uparrow}\rangle - \langle n_{2\downarrow}\rangle + \langle n_{\bar{2}\uparrow}\rangle - \langle n_{\bar{2}\downarrow}\rangle),
\end{aligned} \tag{50}$$

and the orbital polarization per site is defined as

$$\begin{aligned}
l_z &= l_{z1} + l_{z2}, \\
l_{z1} &= \mu_B(\langle n_{1\uparrow}\rangle - \langle n_{\bar{1}\uparrow}\rangle + \langle n_{1\downarrow}\rangle - \langle n_{\bar{1}\downarrow}\rangle), \\
l_{z2} &= 2\mu_B(\langle n_{2\uparrow}\rangle - \langle n_{\bar{2}\uparrow}\rangle + \langle n_{2\downarrow}\rangle - \langle n_{\bar{2}\downarrow}\rangle).
\end{aligned} \tag{51}$$

Introduce the particle numbers of the parallel ($n_{mp}$) and antiparallel ($n_{map}$) states of the spin $\sigma$ and orbital $m$:

$$\begin{aligned}
n_0 &= \langle n_{0\downarrow}\rangle + \langle n_{0\uparrow}\rangle, \\
n_{1p} &= \langle n_{1\uparrow}\rangle + \langle n_{\bar{1}\downarrow}\rangle, \\
n_{1ap} &= \langle n_{1\downarrow}\rangle + \langle n_{\bar{1}\uparrow}\rangle, \\
n_{2p} &= \langle n_{2\uparrow}\rangle + \langle n_{\bar{2}\downarrow}\rangle, \\
n_{2ap} &= \langle n_{2\downarrow}\rangle + \langle n_{\bar{2}\uparrow}\rangle.
\end{aligned} \tag{52}$$

The occupation numbers of different states can be written as

$$\begin{aligned}
\langle n_{\bar{2}\uparrow}\rangle &= \frac{1}{4}(\frac{s_{z2}}{\mu_B} - \frac{l_{z2}}{2\mu_B} + 2n_{2ap}), \\
\langle n_{\bar{2}\downarrow}\rangle &= \frac{1}{4}(-\frac{s_{z2}}{\mu_B} - \frac{l_{z2}}{2\mu_B} + 2n_{2p}), \\
\langle n_{\bar{1}\uparrow}\rangle &= \frac{1}{4}(\frac{s_{z1}}{\mu_B} - \frac{l_{z1}}{\mu_B} + 2n_{1ap}), \\
\langle n_{\bar{1}\downarrow}\rangle &= \frac{1}{4}(-\frac{s_{z1}}{\mu_B} - \frac{l_{z1}}{\mu_B} + 2n_{1p}), \\
\langle n_{0\uparrow}\rangle &= \frac{1}{2}(n_0 + \frac{s_{z0}}{\mu_B}), \\
\langle n_{0\downarrow}\rangle &= \frac{1}{2}(n_0 - \frac{s_{z0}}{\mu_B}), \\
\langle n_{1\uparrow}\rangle &= \frac{1}{4}(\frac{s_{z1}}{\mu_B} + \frac{l_{z1}}{\mu_B} + 2n_{1p}), \\
\langle n_{1\downarrow}\rangle &= \frac{1}{4}(-\frac{s_{z1}}{\mu_B} + \frac{l_{z1}}{\mu_B} + 2n_{1ap}), \\
\langle n_{2\uparrow}\rangle &= \frac{1}{4}(\frac{s_{z2}}{\mu_B} + \frac{l_{z2}}{2\mu_B} + 2n_{2p}), \\
\langle n_{2\downarrow}\rangle &= \frac{1}{4}(-\frac{s_{z2}}{\mu_B} + \frac{l_{z2}}{2\mu_B} + 2n_{2ap}).
\end{aligned} \tag{53}$$

Then the energy $\tilde{E}_{km\sigma}$ in Eq.(49) can be rewritten as

$$
\begin{aligned}
\tilde{\epsilon}_{k\bar{2}\uparrow} =&\epsilon_k + \frac{1}{2}Un_{2p} + \frac{1}{2}U'(2n_{1p}+2n_{1ap}+n_{2p}+n_{2ap}+2n_0) - \frac{1}{2}J_H(n_{1ap}+n_{1p}+n_{2p}+n_0)\\
&-\mu_B\left[h+\frac{U+J_H}{4\mu_B^2}s_{z2}+\frac{2J_H}{4\mu_B^2}(s_{z1}+s_{z0})\right]-(-\lambda_{so}+\frac{U-2U'+J_H}{8\mu_B}l_{z2}),\\
\tilde{\epsilon}_{k2\uparrow} =&\epsilon_k + \frac{1}{2}Un_{2ap} + \frac{1}{2}U'(2n_{1p}+2n_{1ap}+n_{2p}+n_{2ap}+2n_0) - \frac{1}{2}J_H(n_{1ap}+n_{1p}+n_{2ap}+n_0)\\
&-\mu_B\left[h+\frac{U+J_H}{4\mu_B^2}s_{z2}+\frac{2J_H}{4\mu_B^2}(s_{z1}+s_{z0})\right]-(\lambda_{so}-\frac{U-2U'+J_H}{8\mu_B}l_{z2}),\\
\tilde{\epsilon}_{k\bar{1}\uparrow} =&\epsilon_k + \frac{1}{2}Un_{1p} + \frac{1}{2}U'(n_{1p}+n_{1ap}+2n_{2p}+2n_{2ap}+2n_0) - \frac{1}{2}J_H(n_{2ap}+n_{2p}+n_{1p}+n_0)\\
&-\mu_B\left[h+\frac{U+J_H}{4\mu_B^2}s_{z1}+\frac{2J_H}{4\mu_B^2}(s_{z2}+s_{z0})\right]-(-\frac{1}{2}\lambda_{so}+\frac{U-2U'+J_H}{4\mu_B}l_{z1}),\\
\tilde{\epsilon}_{k1\uparrow} =&\epsilon_k + \frac{1}{2}Un_{1p} + \frac{1}{2}U'(n_{1p}+n_{1ap}+2n_{2p}+2n_{2ap}+2n_0) - \frac{1}{2}J_H(n_{2ap}+n_{2p}+n_{1ap}+n_0)\\
&-\mu_B\left[h+\frac{U+J_H}{4\mu_B^2}s_{z1}+\frac{2J_H}{4\mu_B^2}(s_{z2}+s_{z0})\right]-(\frac{1}{2}\lambda_{so}-\frac{U-2U'+J_H}{4\mu_B}l_{z1}),\\
\tilde{\epsilon}_{k0\uparrow} =&\epsilon_k + \frac{1}{2}Un_0 + \frac{1}{2}U'(2n_{1p}+2n_{1ap}+2n_{2p}+2n_{2ap}) - \frac{1}{2}J_H(n_{2ap}+n_{2p}+n_{1ap}+n_{1p})\\
&-\mu_B\left[h+\frac{2U}{4\mu_B^2}s_{z0}+\frac{2J_H}{4\mu_B^2}(s_{z2}+s_{z1})\right],\\
\tilde{\epsilon}_{k0\downarrow} =&\epsilon_k + \frac{1}{2}Un_0 + \frac{1}{2}U'(2n_{1p}+2n_{1ap}+2n_{2p}+2n_{2ap}) - \frac{1}{2}J_H(n_{2ap}+n_{2p}+n_{1ap}+n_{1p})\\
&-\mu_B\left[-h-\frac{2U}{4\mu_B^2}s_{z0}-\frac{2J_H}{4\mu_B^2}(s_{z2}+s_{z1})\right],\\
\tilde{\epsilon}_{k\bar{2}\downarrow} =&\epsilon_k + \frac{1}{2}Un_{2ap} + \frac{1}{2}U'(2n_{1p}+2n_{1ap}+n_{2p}+n_{2ap}+2n_0) - \frac{1}{2}J_H(n_{1ap}+n_{1p}+n_{2ap}+n_0)\\
&-\mu_B\left[-h-\frac{U+J_H}{4\mu_B^2}s_{z2}-\frac{2J_H}{4\mu_B^2}(s_{z1}+s_{z0})\right]-(\lambda_{so}+\frac{U-2U'+J_H}{8\mu_B}l_{z2}),\\
\tilde{\epsilon}_{k2\downarrow} =&\epsilon_k + \frac{1}{2}Un_{2p} + \frac{1}{2}U'(2n_{1p}+2n_{1ap}+n_{2p}+n_{2ap}+2n_0) - \frac{1}{2}J_H(n_{1ap}+n_{1p}+n_{2p}+n_0)\\
&-\mu_B\left[-h-\frac{U+J_H}{4\mu_B^2}s_{z2}-\frac{2J_H}{4\mu_B^2}(s_{z1}+s_{z0})\right]-(-\lambda_{so}-\frac{U-2U'+J_H}{8\mu_B}l_{z2}),\\
\tilde{\epsilon}_{k\bar{1}\downarrow} =&\epsilon_k + \frac{1}{2}Un_{1ap} + \frac{1}{2}U'(n_{1p}+n_{1ap}+2n_{2p}+2n_{2ap}+2n_0) - \frac{1}{2}J_H(n_{2ap}+n_{2p}+n_{1ap}+n_0)\\
&-\mu_B\left[-h-\frac{U+J_H}{4\mu_B^2}s_{z1}-\frac{2J_H}{4\mu_B^2}(s_{z2}+s_{z0})\right]-(\frac{1}{2}\lambda_{so}+\frac{U-2U'+J_H}{4\mu_B}l_{z1}),\\
\tilde{\epsilon}_{k1\downarrow} =&\epsilon_k + \frac{1}{2}Un_{1ap} + \frac{1}{2}U'(n_{1p}+n_{1ap}+2n_{2p}+2n_{2ap}+2n_0) - \frac{1}{2}J_H(n_{2ap}+n_{2p}+n_{1p}+n_0)\\
&-\mu_B\left[-h-\frac{U+J_H}{4\mu_B^2}s_{z1}-\frac{2J_H}{4\mu_B^2}(s_{z2}+s_{z0})\right]-(-\frac{1}{2}\lambda_{so}-\frac{U-2U'+J_H}{4\mu_B}l_{z1}).
\end{aligned}
\tag{54}
$$

### A. Spin Polarization without SOC

It is noted that without the external magnetic field $h$ and SOC $\lambda_{so}$, the four energy bands with spin $\sigma$ ($\uparrow$ and $\downarrow$) and orbital $m$ are degenerate, and the occupation numbers in Eq. (53) have the relation $n_{map} = n_{mp}$. The lattice system has the translational symmetry

$$
\langle n_{m\sigma}\rangle = \frac{1}{N}\sum_i \langle n_{im\sigma}\rangle = \frac{1}{N}\sum_{\mathbf{k}} \langle n_{\mathbf{k}m\sigma}\rangle = \frac{1}{N}\sum_{\mathbf{k}} f\left(\tilde{\epsilon}_{\mathbf{k}m\sigma}\right), \tag{55}
$$

where $f$ is the Fermi distribution function. Then the spin polarization in Eq.(50) can be written as

$$\begin{aligned} s_z &= \mu_B \left( \langle n_{0\uparrow} \rangle - \langle n_{0\downarrow} \rangle + \langle n_{1\uparrow} \rangle - \langle n_{1\downarrow} \rangle + \langle n_{\bar{1}\uparrow} \rangle - \langle n_{\bar{1}\downarrow} \rangle + \langle n_{2\uparrow} \rangle - \langle n_{2\downarrow} \rangle + \langle n_{\bar{2}\uparrow} \rangle - \langle n_{\bar{2}\downarrow} \rangle \right) \\ &= \frac{\mu_B}{N} \sum_{\mathbf{k},m} \left[ f\left(\tilde{\epsilon}_{\mathbf{k}m\uparrow}\right) - f\left(\tilde{\epsilon}_{\mathbf{k}m\downarrow}\right) \right]. \end{aligned} \tag{56}$$

When $h = 0$, the system is in a paramagnetic (PM) state. $f(\tilde{\epsilon}_{\mathbf{k}m\sigma})$ can be expanded according to $h$, which is small compared to the Fermi energy,

$$f\left(\tilde{\epsilon}_{\mathbf{k}m\sigma}\right) \approx f\left(\tilde{\epsilon}_{PM,\mathbf{k}m\sigma}\right) + \left(\tilde{\epsilon}_{\mathbf{k}m\sigma} - \tilde{\epsilon}_{PM,\mathbf{k}m\sigma}\right) \left.\frac{\partial f(E)}{\partial E}\right|_{E=\tilde{\epsilon}_{PM,\mathbf{k}m\sigma}}, \tag{57}$$

where

$$\begin{aligned}
\tilde{\epsilon}_{PM,\mathbf{k}0\uparrow} &= \epsilon_k + \frac{1}{2}Un_0 + \frac{1}{2}U'(2n_{1p} + 2n_{1ap} + 2n_{2p} + 2n_{2ap}) - \frac{1}{2}J_H(n_{2ap} + n_{2p} + n_{1ap} + n_{1p}), \\
\tilde{\epsilon}_{PM,\mathbf{k}0\downarrow} &= \epsilon_k + \frac{1}{2}Un_0 + \frac{1}{2}U'(2n_{1p} + 2n_{1ap} + 2n_{2p} + 2n_{2ap}) - \frac{1}{2}J_H(n_{2ap} + n_{2p} + n_{1ap} + n_{1p}), \\
\tilde{\epsilon}_{PM,\mathbf{k}1\uparrow} &= \epsilon_k + \frac{1}{2}Un_{1p} + \frac{1}{2}U'(n_{1p} + n_{1ap} + 2n_{2p} + 2n_{2ap} + 2n_0) - \frac{1}{2}J_H(n_{2ap} + n_{2p} + n_{1ap} + n_0), \\
\tilde{\epsilon}_{PM,\mathbf{k}1\downarrow} &= \epsilon_k + \frac{1}{2}Un_{1ap} + \frac{1}{2}U'(n_{1p} + n_{1ap} + 2n_{2p} + 2n_{2ap} + 2n_0) - \frac{1}{2}J_H(n_{2ap} + n_{2p} + n_{1p} + n_0), \\
\tilde{\epsilon}_{PM,\mathbf{k}\bar{1}\uparrow} &= \epsilon_k + \frac{1}{2}Un_{1p} + \frac{1}{2}U'(n_{1p} + n_{1ap} + 2n_{2p} + 2n_{2ap} + 2n_0) - \frac{1}{2}J_H(n_{2ap} + n_{2p} + n_{1p} + n_0), \\
\tilde{\epsilon}_{PM,\mathbf{k}\bar{1}\downarrow} &= \epsilon_k + \frac{1}{2}Un_{1ap} + \frac{1}{2}U'(n_{1p} + n_{1ap} + 2n_{2p} + 2n_{2ap} + 2n_0) - \frac{1}{2}J_H(n_{2ap} + n_{2p} + n_{1ap} + n_0), \\
\tilde{\epsilon}_{PM,\mathbf{k}2\uparrow} &= \epsilon_k + \frac{1}{2}Un_{2ap} + \frac{1}{2}U'(2n_{1p} + 2n_{1ap} + n_{2p} + n_{2ap} + 2n_0) - \frac{1}{2}J_H(n_{1ap} + n_{1p} + n_{2ap} + n_0), \\
\tilde{\epsilon}_{PM,\mathbf{k}2\downarrow} &= \epsilon_k + \frac{1}{2}Un_{2p} + \frac{1}{2}U'(2n_{1p} + 2n_{1ap} + n_{2p} + n_{2ap} + 2n_0) - \frac{1}{2}J_H(n_{1ap} + n_{1p} + n_{2p} + n_0), \\
\tilde{\epsilon}_{PM,\mathbf{k}\bar{2}\uparrow} &= \epsilon_k + \frac{1}{2}Un_{2p} + \frac{1}{2}U'(2n_{1p} + 2n_{1ap} + n_{2p} + n_{2ap} + 2n_0) - \frac{1}{2}J_H(n_{1ap} + n_{1p} + n_{2p} + n_0), \\
\tilde{\epsilon}_{PM,k\bar{2}\downarrow} &= \epsilon_k + \frac{1}{2}Un_{2ap} + \frac{1}{2}U'(2n_{1p} + 2n_{1ap} + n_{2p} + n_{2ap} + 2n_0) - \frac{1}{2}J_H(n_{1ap} + n_{1p} + n_{2ap} + n_0).
\end{aligned} \tag{58}$$

When $h = 0$, $n_{map} = n_{mp}$, it has

$$\mu_B \sum_{\mathbf{k},m} \left[ f\left(\tilde{\epsilon}_{PM,km\uparrow}\right) - f\left(\tilde{\epsilon}_{PM,km\downarrow}\right) \right] = 0. \tag{59}$$

The spin polarization in Eq.(56) can be calculated up to the first order of $h$,

$$\begin{aligned}
s_z \approx& \left[ \mu_B^2 h + \frac{2U}{4} s_{z0} + \frac{2J_H}{4}(s_{z1} + s_{z2}) \right] \int_0^\infty \left[ -\frac{\partial f(E)}{\partial E} \right] \left[ \rho_{0\uparrow}(E) + \rho_{0\downarrow}(E) \right] dE \\
&+ \left[ \mu_B^2 h + \frac{U + J_H}{4} s_{z2} + \frac{2J_H}{4}(s_{z1} + s_{z0}) \right] \int_0^\infty \left[ -\frac{\partial f(E)}{\partial E} \right] \left[ \rho_{2\uparrow}(E) + \rho_{\bar{2}\uparrow}(E) + \rho_{2\downarrow}(E) + \rho_{\bar{2}\downarrow}(E) \right] dE \\
&+ \left[ \mu_B^2 h + \frac{U + J_H}{4} s_{z1} + \frac{2J_H}{4}(s_{z2} + s_{z0}) \right] \int_0^\infty \left[ -\frac{\partial f(E)}{\partial E} \right] \left[ \rho_{1\uparrow}(E) + \rho_{\bar{1}\uparrow}(E) + \rho_{1\downarrow}(E) + \rho_{\bar{1}\downarrow}(E) \right] dE.
\end{aligned} \tag{60}$$

Then

$$\begin{aligned}
s_z =& \left[ \mu_B^2 h + \frac{2U}{4} s_{z0} + \frac{2J_H}{4}(s_{z1} + s_{z2}) \right] 2\rho_0 \\
&+ \left[ \mu_B^2 h + \frac{U + J_H}{4} s_{z2} + \frac{2J_H}{4}(s_{z1} + s_{z0}) \right] 4\rho_2 \\
&+ \left[ \mu_B^2 h + \frac{U + J_H}{4} s_{z1} + \frac{2J_H}{4}(s_{z2} + s_{z0}) \right] 4\rho_1,
\end{aligned} \tag{61}$$

where

$$\rho_0 =\frac{1}{2}\int_0^\infty \left[-\frac{\partial f(E)}{\partial E}\right][\rho_{0\uparrow}(E)+\rho_{0\downarrow}(E)]\,dE,$$
$$\rho_1 =\frac{1}{4}\int_0^\infty \left[-\frac{\partial f(E)}{\partial E}\right]\left[\rho_{1\uparrow}(E)+\rho_{\bar{1}\uparrow}(E)+\rho_{1\downarrow}(E)+\rho_{\bar{1}\downarrow}(E)\right]dE, \tag{62}$$
$$\rho_2 =\frac{1}{4}\int_0^\infty \left[-\frac{\partial f(E)}{\partial E}\right]\left[\rho_{2\uparrow}(E)+\rho_{\bar{2}\uparrow}(E)+\rho_{2\downarrow}(E)+\rho_{\bar{2}\downarrow}(E)\right]dE.$$

which is the average density of states for the orbitals 0, ±1, ±2, respectively. For the degenerated five orbitals, $\rho_0=\rho_1=\rho_2$. Then the spin polarization per site $s_z$ defined in Eq. (50) can be calculated as

$$s_z=\frac{10\mu_B^2\rho_0}{1-(U+4J_H)\rho_0}h. \tag{63}$$

The magnetic susceptibility can be written as

$$\chi=\frac{\partial s_z}{\partial h}=\frac{10\mu_B^2\rho_0}{1-(U+4J_H)\rho_0} \tag{64}$$

The instability condition of the spin polarization in ferromagnets can be obtained as

$$(U+4J_H)\rho_0>1. \tag{65}$$

## B. Spin Polarization with SOC

If we consider the SOC, the spin polarization in Eq.(56) can be calculated up to the first order of $h$ and $\lambda_{so}$.

$$\begin{aligned}
s_z=&\left[\mu_B^2h+\frac{2U}{4}s_{z0}+\frac{2J_H}{4}(s_{z1}+s_{z2})\right]\int_0^\infty\left[-\frac{\partial f(E)}{\partial E}\right][\rho_{0\uparrow}(E)+\rho_{0\downarrow}(E)]\,dE\\
&+\left[\mu_B^2h+\frac{U+J_H}{4}s_{z2}+\frac{2J_H}{4}(s_{z1}+s_{z0})\right]\int_0^\infty\left[-\frac{\partial f(E)}{\partial E}\right]\left[\rho_{2\uparrow}(E)+\rho_{\bar{2}\uparrow}(E)+\rho_{2\downarrow}(E)+\rho_{\bar{2}\downarrow}(E)\right]dE\\
&+\left[\mu_B^2h+\frac{U+J_H}{4}s_{z1}+\frac{2J_H}{4}(s_{z2}+s_{z0})\right]\int_0^\infty\left[-\frac{\partial f(E)}{\partial E}\right]\left[\rho_{1\uparrow}(E)+\rho_{\bar{1}\uparrow}(E)+\rho_{1\downarrow}(E)+\rho_{\bar{1}\downarrow}(E)\right]dE\\
&+\frac{1}{2}\lambda_{so}\mu_B\int_0^\infty\left[-\frac{\partial f(E)}{\partial E}\right]\left[-\rho_{\bar{1}\uparrow}(E)-\rho_{1\downarrow}(E)+\rho_{1\uparrow}(E)+\rho_{\bar{1}\downarrow}(E)\right]dE\\
&+\lambda_{so}\mu_B\int_0^\infty\left[-\frac{\partial f(E)}{\partial E}\right]\left[-\rho_{\bar{2}\uparrow}(E)-\rho_{2\downarrow}(E)+\rho_{2\uparrow}(E)+\rho_{\bar{2}\downarrow}(E)\right]dE.
\end{aligned} \tag{66}$$

In Eq.(66), the term proportional to the orbital polarization $l_z$ has been ignored, since $l_z$ is a small value compared to the spin polarization $s_z$. Then, it has

$$s_z\approx 10\mu_B^2h\rho_0+(U+4J_H)(s_{z1}+s_{z2}+s_{z0})\rho_0+\lambda_{so}\mu_B(\rho_{1p-ap}+2\rho_{2p-ap}), \tag{67}$$

where

$$\rho_{1p-ap}=\frac{1}{2}\int_0^\infty\left[-\frac{\partial f(E)}{\partial E}\right]\left[\rho_{1\uparrow}(E)+\rho_{\bar{1}\downarrow}(E)-\rho_{\bar{1}\uparrow}(E)-\rho_{1\downarrow}(E)\right]dE,$$
$$\rho_{2p-ap}=\frac{1}{2}\int_0^\infty\left[-\frac{\partial f(E)}{\partial E}\right]\left[\rho_{2\uparrow}(E)+\rho_{\bar{2}\downarrow}(E)-\rho_{\bar{2}\uparrow}(E)-\rho_{2\downarrow}(E)\right]dE. \tag{68}$$

which is the difference of the density of sates with parallel spin $\sigma$ and orbital $m$ and that with antiparallel $\sigma$ and $m$. Then the spin polarization per site can be calculated as

$$s_z=\frac{10\mu_B^2\rho_0h+\lambda_{so}\mu_B(\rho_{1p-ap}+2\rho_{2p-ap})}{1-(U+4J_H)\rho_0}. \tag{69}$$

The magnetic susceptibility $\chi$ is the same as in Eq. (64), and the instability condition of the spin polarization with SOC is the same as that without SOC in Eq. (65).

### C. Orbital Polarization from SOC

Similarly, by Eq.(55) the orbital polarization in Eq.(51) can be expressed as

$$\begin{aligned} l_z &= \mu_B \left( \langle n_{1\uparrow} \rangle - \langle n_{\bar{1}\uparrow} \rangle + \langle n_{1\downarrow} \rangle - \langle n_{\bar{1}\downarrow} \rangle \right) + 2\mu_B \left( \langle n_{2\uparrow} \rangle - \langle n_{\bar{2}\uparrow} \rangle + \langle n_{2\downarrow} \rangle - \langle n_{\bar{2}\downarrow} \rangle \right) \\ &= \frac{\mu_B}{N} \sum_k \left[ 2f\left(\tilde{\epsilon}_{k2\uparrow}\right) - 2f\left(\tilde{\epsilon}_{k\bar{2}\uparrow}\right) + 2f\left(\tilde{\epsilon}_{k2\downarrow}\right) - 2f\left(\tilde{\epsilon}_{k\bar{2}\downarrow}\right) + f\left(\tilde{\epsilon}_{k1\uparrow}\right) - f\left(\tilde{\epsilon}_{k\bar{1}\uparrow}\right) + f\left(\tilde{\epsilon}_{k1\downarrow}\right) - f\left(\tilde{\epsilon}_{k\bar{1}\downarrow}\right) \right]. \end{aligned} \tag{70}$$

On the basis of ferromagnetic (FM) state, the SOC can be regarded smaller than the Fermi energy[1], so $f(\tilde{\epsilon}_{\mathbf{k}m\sigma})$ can be expanded according to $\lambda_{so}$

$$f\left(\tilde{\epsilon}_{km\sigma}\right) \approx f\left(\tilde{\epsilon}_{FM,km\sigma}\right) + \left[\frac{\partial f(E)}{\partial E}\right]_{E=\tilde{\epsilon}_{FM,km\sigma}} \left(\tilde{\epsilon}_{km\sigma} - \tilde{\epsilon}_{FM,km\sigma}\right), \tag{71}$$

where

$$\begin{aligned}
\tilde{\epsilon}_{FM,\mathbf{k}1\uparrow} &= \epsilon_k + \frac{1}{2}Un_{1p} + \frac{1}{2}U'(n_{1p} + n_{1ap} + 2n_{2p} + 2n_{2ap} + 2n_0) - \frac{1}{2}J_H(n_{2ap} + n_{2p} + n_{1ap} + n_0) \\
&\quad - \mu_B\left[h + \frac{U+J_H}{4\mu_B^2}s_{z1} + \frac{2J_H}{4\mu_B^2}(s_{z2} + s_{z0})\right], \\
\tilde{\epsilon}_{FM,\mathbf{k}1\downarrow} &= \epsilon_k + \frac{1}{2}Un_{1ap} + \frac{1}{2}U'(n_{1p} + n_{1ap} + 2n_{2p} + 2n_{2ap} + 2n_0) - \frac{1}{2}J_H(n_{2ap} + n_{2p} + n_{1p} + n_0) \\
&\quad - \mu_B\left[-h - \frac{U+J_H}{4\mu_B^2}s_{z1} - \frac{2J_H}{4\mu_B^2}(s_{z2} + s_{z0})\right], \\
\tilde{\epsilon}_{FM,\mathbf{k}\bar{1}\uparrow} &= \epsilon_k + \frac{1}{2}Un_{1p} + \frac{1}{2}U'(n_{1p} + n_{1ap} + 2n_{2p} + 2n_{2ap} + 2n_0) - \frac{1}{2}J_H(n_{2ap} + n_{2p} + n_{1p} + n_0) \\
&\quad - \mu_B\left[h + \frac{U+J_H}{4\mu_B^2}s_{z1} + \frac{2J_H}{4\mu_B^2}(s_{z2} + s_{z0})\right], \\
\tilde{\epsilon}_{FM,\mathbf{k}\bar{1}\downarrow} &= \epsilon_k + \frac{1}{2}Un_{1ap} + \frac{1}{2}U'(n_{1p} + n_{1ap} + 2n_{2p} + 2n_{2ap} + 2n_0) - \frac{1}{2}J_H(n_{2ap} + n_{2p} + n_{1ap} + n_0) \\
&\quad - \mu_B\left[-h - \frac{U+J_H}{4\mu_B^2}s_{z1} - \frac{2J_H}{4\mu_B^2}(s_{z2} + s_{z0})\right], \\
\tilde{\epsilon}_{FM,\mathbf{k}2\uparrow} &= \epsilon_k + \frac{1}{2}Un_{2ap} + \frac{1}{2}U'(2n_{1p} + 2n_{1ap} + n_{2p} + n_{2ap} + 2n_0) - \frac{1}{2}J_H(n_{1ap} + n_{1p} + n_{2ap} + n_0) \\
&\quad - \mu_B\left[h + \frac{U+J_H}{4\mu_B^2}s_{z2} + \frac{2J_H}{4\mu_B^2}(s_{z1} + s_{z0})\right], \\
\tilde{\epsilon}_{FM,\mathbf{k}2\downarrow} &= \epsilon_k + \frac{1}{2}Un_{2p} + \frac{1}{2}U'(2n_{1p} + 2n_{1ap} + n_{2p} + n_{2ap} + 2n_0) - \frac{1}{2}J_H(n_{1ap} + n_{1p} + n_{2p} + n_0) \\
&\quad - \mu_B\left[-h - \frac{U+J_H}{4\mu_B^2}s_{z2} - \frac{2J_H}{4\mu_B^2}(s_{z1} + s_{z0})\right], \\
\tilde{\epsilon}_{FM,\mathbf{k}\bar{2}\uparrow} &= \epsilon_k + \frac{1}{2}Un_{2p} + \frac{1}{2}U'(2n_{1p} + 2n_{1ap} + n_{2p} + n_{2ap} + 2n_0) - \frac{1}{2}J_H(n_{1ap} + n_{1p} + n_{2p} + n_0) \\
&\quad - \mu_B\left[h + \frac{U+J_H}{4\mu_B^2}s_{z2} + \frac{2J_H}{4\mu_B^2}(s_{z1} + s_{z0})\right], \\
\tilde{\epsilon}_{FM,k\bar{2}\downarrow} &= \epsilon_k + \frac{1}{2}Un_{2ap} + \frac{1}{2}U'(2n_{1p} + 2n_{1ap} + n_{2p} + n_{2ap} + 2n_0) - \frac{1}{2}J_H(n_{1ap} + n_{1p} + n_{2ap} + n_0) \\
&\quad - \mu_B\left[-h - \frac{U+J_H}{4\mu_B^2}s_{z2} - \frac{2J_H}{4\mu_B^2}(s_{z1} + s_{z0})\right].
\end{aligned} \tag{72}$$

By Eq.(54) it yields

$$\tilde{\epsilon}_{km\sigma} - \tilde{\epsilon}_{FM,km\sigma} = -\frac{1}{2}m\left(\sigma\lambda_{so} - \frac{U - 2U' + J_H}{2\mu_B m^2} l_{zm}\right). \tag{73}$$

When $\lambda_{so} = 0$, $n_{map} = n_{mp}$, we have

$$\frac{\mu_B}{N} \sum_k \left[ 2f\left(\tilde{\epsilon}_{k2\uparrow}\right) - 2f\left(\tilde{\epsilon}_{k\bar{2}\uparrow}\right) + 2f\left(\tilde{\epsilon}_{k2\downarrow}\right) - 2f\left(\tilde{\epsilon}_{k\bar{2}\downarrow}\right) + f\left(\tilde{\epsilon}_{k1\uparrow}\right) - f\left(\tilde{\epsilon}_{k\bar{1}\uparrow}\right) + f\left(\tilde{\epsilon}_{k1\downarrow}\right) - f\left(\tilde{\epsilon}_{k\bar{1}\downarrow}\right) \right] = 0. \tag{74}$$

The orbital polarization in Eq.(70) can be calculated up to the first order of $\lambda_{so}$,

$$\begin{aligned} l_z \approx & \frac{1}{2}\lambda_{so}\mu_B \int_0^\infty \left[-\frac{\partial f(E)}{\partial E}\right]\left[\rho_{\bar{1}\uparrow}(E)+\rho_{1\uparrow}(E)-\rho_{1\downarrow}(E)-\rho_{\bar{1}\downarrow}(E)\right] dE \\ & +2\lambda_{so}\mu_B \int_0^\infty \left[-\frac{\partial f(E)}{\partial E}\right]\left[\rho_{\bar{2}\uparrow}(E)+\rho_{2\uparrow}(E)-\rho_{2\downarrow}(E)-\rho_{\bar{2}\downarrow}(E)\right] dE \\ & +\left[\frac{2U'-U-J_H}{4}l_{z2}\right]\int_0^\infty \left[-\frac{\partial f(E)}{\partial E}\right]\left[\rho_{2\uparrow}(E)+\rho_{\bar{2}\uparrow}(E)+\rho_{2\downarrow}(E)+\rho_{\bar{2}\downarrow}(E)\right] dE \\ & +\left[\frac{2U'-U-J_H}{4}l_{z1}\right]\int_0^\infty \left[-\frac{\partial f(E)}{\partial E}\right]\left[\rho_{1\uparrow}(E)+\rho_{\bar{1}\uparrow}(E)+\rho_{1\downarrow}(E)+\rho_{\bar{1}\downarrow}(E)\right] dE. \end{aligned} \tag{75}$$

Then

$$l_z \approx \mu_B\lambda_{so}(\rho_{1s}+4\rho_{2s})+(2U'-U-J_H)\,\rho_0 l_z, \tag{76}$$

where

$$\begin{aligned} \rho_{1s} =& \frac{1}{2N}\int_0^\infty \left[-\frac{\partial f(E)}{\partial E}\right]\left[\rho_{1\uparrow}(E)+\rho_{\bar{1}\uparrow}(E)-\rho_{1\downarrow}(E)-\rho_{\bar{1}\downarrow}(E)\right] dE, \\ \rho_{2s} =& \frac{1}{2N}\int_0^\infty \left[-\frac{\partial f(E)}{\partial E}\right]\left[\rho_{2\uparrow}(E)+\rho_{\bar{2}\uparrow}(E)-\rho_{2\downarrow}(E)-\rho_{\bar{2}\downarrow}(E)\right] dE, \end{aligned} \tag{77}$$

which is the average spin polarized density of states for the orbitals $\pm 1$ and $\pm 2$, respectively. Thus, the orbital polarization per site can be calculated as

$$l_z = \frac{\mu_B(\rho_{1s}+4\rho_{2s})}{1-(2U'-U-J_H)\,\rho_0}\lambda_{so}, \tag{78}$$

where $\rho_0$ is given by Eq.(62). And Eq.(51) can be rewritten as

$$l_z = \mu_B(\rho_{1s}+4\rho_{2s})\lambda_{so}^{\rm eff}, \tag{79}$$

where the effective SOC $\lambda_{so}^{\rm eff}$ is expressed as

$$\lambda_{so}^{\rm eff} = \frac{\lambda_{so}}{1-(2U'-U-J_H)\,\rho_0}. \tag{80}$$

The instability condition of orbital polarization from SOC in ferromagnets can be obtained as

$$(2U'-U-J_H)\rho_0 > 1. \tag{81}$$

* gubo@ucas.ac.cn
† gsu@ucas.ac.cn
[1] A. Fert and O. Jaoul, Phys. Rev. Lett. **28**, 303 (1972).
